# Supplementary material for: Dielectric properties of aqueous electrolytes at the nanoscale
Source: arXiv:2303.14846 source file (2025-04-24)
Supplement: Supplementary file 1 [file SI.pdf]

# Supplementary Materials for Dielectric properties of aqueous electrolytes at the nanoscale

Maximilian R. Becker and Roland R. Netz\*

*Fachbereich Physik, Freie Universität Berlin, Arnimallee 14, Berlin, 14195, Germany*

Philip Loche

*Laboratory of Computational Science and Modeling, IMX,*

*École Polytechnique Fédérale de Lausanne, 1015 Lausanne, Switzerland and*

*Fachbereich Physik, Freie Universität Berlin, Arnimallee 14, Berlin, 14195, Germany*

Douwe Jan Bonthuis

*Institute of Theoretical and Computational Physics, Graz University of Technology, Graz, Austria*

Dominique Mouhanna

*Sorbonne Université, CNRS, Laboratoire de Physique Théorique de*

*la Matière Condensée (LPTMC, UMR 7600), F-75005 Paris, France*

Hélène Berthoumieux†

*Gulliver, CNRS, École Supérieure de Physique et Chimie Industrielles de Paris,*

*Paris Sciences et Lettres Research University, Paris 75005, France*

## Contents

|                                                                                    |           |
|------------------------------------------------------------------------------------|-----------|
| <b>S1. Supplementary information for the field theory model</b>                    | <b>1</b>  |
| S1.1. Model for nonlocal dielectric properties of water                            | 1         |
| S1.2. Derivation of $\Xi$ , the partition function in the grand canonical ensemble | 2         |
| S1.3. Mean field ( $\psi$ , $P$ ) for the linear and nonlinear models              | 4         |
| S1.4. Gaussian susceptibility for an electrolyte                                   | 4         |
| S1.5. Susceptibility for Gaussian model in real space                              | 5         |
| S1.6. One-loop free energy expansion                                               | 7         |
| S1.7. One-loop correction for the inverse susceptibility                           | 7         |
| S1.8. Linear dependence of $\chi^{-1,1}(q)$ in salt concentration $c$              | 9         |
| <b>S2. Supplementary information for molecular dynamic simulation</b>              | <b>10</b> |
| S2.1. Methods                                                                      | 10        |
| <b>References</b>                                                                  | <b>12</b> |

## S1. SUPPLEMENTARY INFORMATION FOR THE FIELD THEORY MODEL

### S1.1. Model for nonlocal dielectric properties of water

We consider a field theory (FT) model describing the dielectric properties of water at the nanoscale. The electrostatic energy of the system is written as a functional of the polarization  $\mathcal{P}$  as follows [1]:

$$\mathcal{U}_{\text{el}}[\mathcal{P}] = \frac{1}{2} \int d\mathbf{r} d\mathbf{r}' \frac{\nabla \cdot \mathcal{P}(\mathbf{r}) \nabla \cdot \mathcal{P}(\mathbf{r}')}{4\pi\epsilon_0 |\mathbf{r} - \mathbf{r}'|} + \mathcal{U}_{\text{conf}}^{\text{G}}[\mathcal{P}]. \quad (\text{S1})$$

---

\*rnetz@physik.fu-berlin.de

†helene.berthoumieux@espci.fr

The first term corresponds to the bare Coulomb interactions between the partial charges  $-\nabla \cdot \mathcal{P}(\mathbf{r})$  of the fluid and the second term  $\mathcal{U}_{\text{conf}}^G$  - where the index G stands for Gaussian - is a phenomenological configuration energy. It can be written following a Landau-Ginzburg approach. We consider it here up to the second spatial derivative in the polarization  $\mathcal{P}$  to reproduce the dielectric response of water and set

$$\begin{aligned} \mathcal{U}_{\text{conf}}^G[\mathcal{P}] &= \frac{1}{2\epsilon_0} \int d\mathbf{r} d\mathbf{r}' \mathcal{P}(\mathbf{r}) \cdot K(\mathbf{r} - \mathbf{r}') \cdot \mathcal{P}(\mathbf{r}') \quad \text{with} \\ \mathcal{P}(\mathbf{r}) K(\mathbf{r} - \mathbf{r}') \mathcal{P}(\mathbf{r}') &= \left[ K \mathcal{P}(\mathbf{r})^2 + \kappa_l (\nabla \cdot \mathcal{P}(\mathbf{r}))^2 + \kappa_t (\nabla \times \mathcal{P}(\mathbf{r}))^2 + \alpha (\nabla (\nabla \cdot \mathcal{P}(\mathbf{r})))^2 \right] \delta(\mathbf{r} - \mathbf{r}'). \end{aligned} \quad (\text{S2})$$

Note that as we consider bulk water which is homogeneous and isotropic, the two-point kernel  $K$  depends simply on the distance  $\mathbf{r} - \mathbf{r}'$ . We introduce the two-point dielectric susceptibility  $\chi^w(\mathbf{r} - \mathbf{r}')$  defined as:

$$\mathcal{U}_{\text{el}}[\mathcal{P}] = \frac{1}{2\epsilon_0} \int d\mathbf{r} d\mathbf{r}' \mathcal{P}(\mathbf{r}) (\chi^w(\mathbf{r} - \mathbf{r}'))^{-1} \mathcal{P}(\mathbf{r}') \quad (\text{S3})$$

where the superscript w stands for water considered here as a pure solvent. The matrix  $\chi^w$  can be decomposed in Fourier space into a longitudinal  $\chi_{\parallel}^w$  and a transverse  $\chi_{\perp}^w$  function, such that

$$\begin{aligned} \chi_{ij}^w(\mathbf{q}) &= \chi_{\parallel}^w(q) \frac{q_i q_j}{q^2} + \chi_{\perp}^w(q) (\delta_{ij} - \frac{q_i q_j}{q^2}) \\ \chi_{\parallel}^w(q) &= \frac{1}{1 + K + \kappa_l q^2 + \alpha q^4}, \quad \chi_{\perp}^w(q) = \frac{1}{K + \kappa_t q^2}. \end{aligned} \quad (\text{S4})$$

The figure S1 shows the MD simulated longitudinal a) and transverse b) response function for the 3 charge water model TIP4p/ε [2] (blue markers). MD data show an overresponse of the system  $\chi_{\parallel}^w(q) > 1$  around  $q=3 \text{ \AA}^{-1}$ , which corresponds to a negative permittivity, as  $\epsilon(q)$  obeys  $\epsilon(q) = 1/(1 - \chi_{\parallel}^w(q))$  [3]. This overscreening phenomenon can be attributed to the H-bond network structuring water at short range [4]. Note that the secondary peak for  $q > 4 \text{ \AA}^{-1}$  corresponds to intramolecular correlations and to length scales that are not addressed in this study. The transverse susceptibility is also extracted from MD simulations and shows a spectrum of simpler shape, as it monotonously decays.

The minimal model given in Eq. (S2) can reproduce these main features. For the longitudinal susceptibility, we consider the case ( $\kappa_l < 0$ ,  $\alpha > 0$ ). The value of the parameters  $K$ ,  $\kappa_l$ , and  $\alpha$ , are adjusted to fit the bulk value,  $\chi_{\parallel}^w(0)$ , the position and the value of the maximum of  $\chi_{\parallel}^w(q)$  of the the MD simulated response. The parameter  $\kappa_t$  is chosen to fit the decay of MD data. Fig. S1 shows the FT response functions (black line). The values of the parameters are given in the caption.

The longitudinal susceptibility  $\chi_{\parallel}^w(q)$  is associated with two correlation lengths: a longitudinal decay,  $\lambda_d$  and an oscillation length  $\lambda_o$ , defined as the imaginary and real part of the inverse of the poles of the function. The transverse susceptibility  $\chi_{\perp}^w(q)$  is associated with a decay length  $\lambda_t$  which is the inverse of its pole. Their expressions obey:

$$\lambda_d = \frac{2\sqrt{\alpha}}{\sqrt{2\sqrt{\alpha}(1+K)} + \kappa_l}, \quad \lambda_t = \sqrt{\frac{\kappa_t}{K}}, \quad \lambda_o = \frac{4\pi\sqrt{\alpha}}{\sqrt{2\sqrt{\alpha}(1+K)} - \kappa_l}. \quad (\text{S5})$$

The polarization-polarization correlation function in the real space can be derived by Fourier transforming the susceptibility given in Eq.(S4) and has been studied in a previous work [5]. Using the estimated values of the parameters we get a longitudinal decay length  $\lambda_d=4.7 \text{ \AA}$ , an oscillating length  $\lambda_o=2.1 \text{ \AA}$ , and a transverse decay length,  $\lambda_t=1.05 \text{ \AA}$ .

### S1.2. Derivation of $\Xi$ , the partition function in the grand canonical ensemble

In this subsection, we present the main steps of the derivation of the partition function  $\Xi^G$  in the grand canonical ensemble. We start from the partition function of the canonical ensemble,  $\mathcal{Z}^G$ ,

$$\mathcal{Z}^G = \frac{1}{N_+!} \frac{1}{N_-!} \left[ \prod_{i=1}^{N_+} \int d\mathbf{r}_i^+ \right] \left[ \prod_{j=1}^{N_-} \int d\mathbf{r}_j^- \right] \int \mathcal{D}[\mathcal{P}] e^{-\beta \mathcal{U}_{\text{conf}}^G[\mathcal{P}]} e^{-\frac{\beta}{2} \int d\mathbf{r} d\mathbf{r}' \rho_{\text{tot}}(\mathbf{r}) v(\mathbf{r} - \mathbf{r}') \rho_{\text{tot}}(\mathbf{r}')} \quad (\text{S6})$$

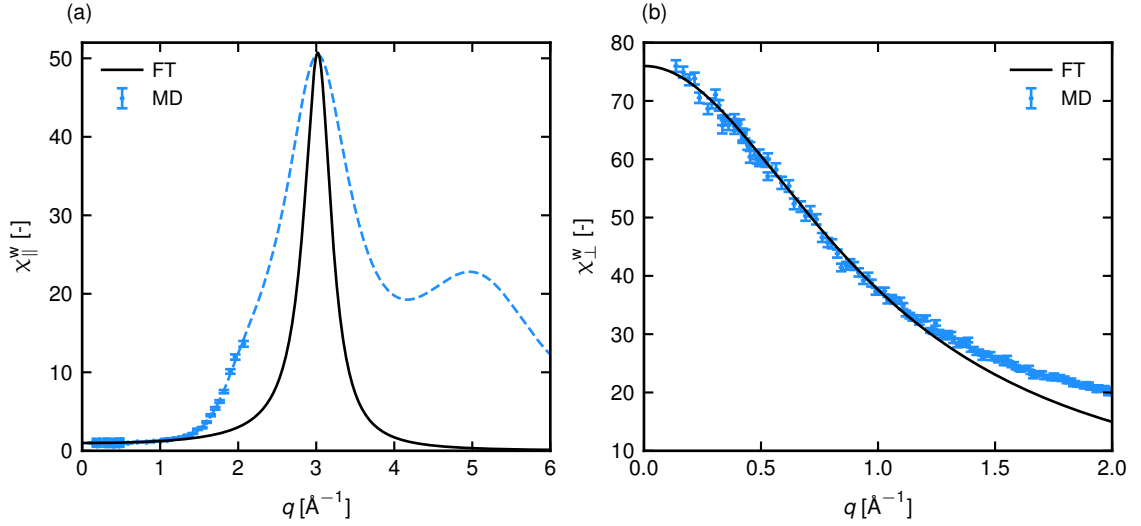

FIG. S1: MD simulated and FT derived susceptibilities for bulk water. (a) Longitudinal and (b) transverse susceptibilities in Fourier space from FT model Eq. (S4) and from MD simulations (details given in S2). The parameter values of the FT model are  $K = 1/76$ ,  $\kappa_l = -0.218 \text{ \AA}^{-2}$ ,  $\alpha = 0.012 \text{ \AA}^{-4}$  and  $\kappa_t = 0.013 \text{ \AA}^{-2}$ .

with  $v(\mathbf{r} - \mathbf{r}') = 1/4\pi\epsilon_0|\mathbf{r} - \mathbf{r}'|$ , the Coulomb potential and  $\rho_{\text{tot}}(\mathbf{r}) = \rho(\mathbf{r}) - \nabla \cdot \mathcal{P}(\mathbf{r})$ . We introduce an auxiliary field  $\Phi$  and perform a Hubbard-Stratonovich transformation using the relation  $v(\mathbf{r} - \mathbf{r}')^{-1} = -\epsilon_0 \nabla^2 \delta(\mathbf{r} - \mathbf{r}')$  [6]. Dropping the prefactor, we get

$$\mathcal{Z}^G = \frac{1}{N_+!} \frac{1}{N_-!} \left[ \prod_{i=1}^{N_+} \int d\mathbf{r}_i^+ \right] \left[ \prod_{j=1}^{N_-} \int d\mathbf{r}_j^- \right] \int \mathcal{D}[\mathcal{P}] e^{-\beta \mathcal{U}_{\text{conf}}^G[\mathcal{P}]} \int \mathcal{D}[\Phi] e^{-\frac{\beta}{2} \int d\mathbf{r} \epsilon_0 (\nabla \Phi)^2 - i\beta \int d\mathbf{r} \Phi(\mathbf{r}) (\rho(\mathbf{r}) - \nabla \cdot \mathcal{P}(\mathbf{r}))}. \quad (\text{S7})$$

Introducing the expression of the charge density  $\rho(\mathbf{r}) = \sum_{i=1}^{N_+} e \delta(\mathbf{r} - \mathbf{r}_i^+) - \sum_{j=1}^{N_-} e \delta(\mathbf{r} - \mathbf{r}_j^-)$ , we get,

$$\begin{aligned} \mathcal{Z}^G &= \int \mathcal{D}[\Phi] \frac{1}{N_+!} \left( \int d\mathbf{r} e^{-i\beta e \Phi(\mathbf{r})} \right)^{N_+} \frac{1}{N_-!} \left( \int d\mathbf{r} e^{i\beta e \Phi(\mathbf{r})} \right)^{N_-} e^{-\frac{\beta}{2} \int d\mathbf{r} \epsilon_0 (\nabla \Phi(\mathbf{r}))^2} \\ &\times \int \mathcal{D}[\mathcal{P}] e^{-\beta \mathcal{U}_{\text{conf}}^G[\mathcal{P}]} e^{-i\beta \int d\mathbf{r} \Phi(\mathbf{r}) (-\nabla \cdot \mathcal{P}(\mathbf{r}))} \end{aligned} \quad (\text{S8})$$

The partition function is brought into a more manageable form by going to the grand canonical ensemble, where we get

$$\begin{aligned} \Xi^G &= \sum_{N_+=0}^{\infty} \frac{e^{-\beta \mu_+ N_+}}{N_+!} \left( \int d\mathbf{r} e^{-i\beta e \Phi(\mathbf{r})} \right)^{N_+} \times \sum_{N_-=0}^{\infty} \frac{e^{-\beta \mu_- N_-}}{N_-!} \left( \int d\mathbf{r} e^{i\beta e \Phi(\mathbf{r})} \right)^{N_-} \\ &\times \int \mathcal{D}[\mathcal{P}] e^{-\beta \mathcal{U}_{\text{conf}}^G[\mathcal{P}]} \int \mathcal{D}[\Phi] e^{-\frac{\beta}{2} \int d\mathbf{r} \epsilon_0 (\nabla \Phi(\mathbf{r}))^2 - i\beta \int d\mathbf{r} \Phi(\mathbf{r}) (-\nabla \cdot \mathcal{P}(\mathbf{r}))}, \end{aligned} \quad (\text{S9})$$

with  $\mu_i$ , ( $i = +, -$ ), the chemical potential for cations and anions. We introduce the field  $\Psi = i\Phi$  that can be identified as the electrostatic potential [6], we perform the sums over  $N_{\pm}$  and identify the action  $F_u^G[\Psi, \mathcal{P}]$ , such that

$$\Xi^G = \int \mathcal{D}[\mathcal{P}] \mathcal{D}[\Psi] e^{-\beta F_u^G[\mathcal{P}, \Psi]}. \quad (\text{S10})$$

Setting  $e^{-\beta \mu_{\pm}} = n$ , the ionic density, we obtain

$$F_u^G[\mathcal{P}, \Psi] = \mathcal{U}_{\text{conf}}^G[\mathcal{P}] - \int d\mathbf{r} \left( \frac{\epsilon_0}{2} (\nabla \Psi)^2 - \Psi \nabla \cdot \mathcal{P} - \frac{2n}{\beta} \cosh(\beta \Psi e) \right). \quad (\text{S11})$$

### S1.3. Mean field $(\psi, \mathbf{P})$ for the linear and nonlinear models

In this subsection, we derive  $(\psi, \mathbf{P})$ , the fields minimizing the action  $F_u^G$  given in Eq. (S11), and the action  $F_u$  obtained by replacing  $\mathcal{U}_{\text{conf}}^G$  in Eq. (S11) by the non Gaussian configuration energy,

$$\mathcal{U}_{\text{conf}}[\mathbf{P}] = \frac{1}{2\epsilon_0} \int d\mathbf{r} \left[ \gamma(\mathbf{P}(\mathbf{r})^2 + P_0^2)^2 + \kappa_l(\nabla \cdot \mathbf{P}(\mathbf{r}))^2 + \kappa_t(\nabla \times \mathbf{P}(\mathbf{r}))^2 + \alpha(\nabla(\nabla \cdot \mathbf{P}(\mathbf{r})))^2 \right]. \quad (\text{S12})$$

The mean fields obey the following equations:

$$\frac{\delta F_u^k}{\delta \Psi} \Big|_{\mathbf{P}} = 0, \quad \frac{\delta F_u^k}{\delta \mathcal{P}_i} \Big|_{\Psi} = 0, \quad k = G, \emptyset, \quad i = x, y, z. \quad (\text{S13})$$

The functional derivative with respect to  $\Psi$  gives:

$$\frac{\delta F_u^k}{\delta \Psi} = \epsilon_0 \Delta \Psi - \nabla \cdot \mathbf{P} - 2en \sinh(\beta e \Psi), \quad (\text{S14})$$

The functional derivative with respect to  $\mathcal{P}_i$  leads to

$$\frac{\delta F_u^G}{\delta \mathcal{P}_i} = \frac{1}{\epsilon_0} \left( K \mathcal{P}_i - \kappa_l \partial_i \nabla \cdot \mathbf{P} + \kappa_t (\partial_i \nabla \cdot \mathbf{P} - \Delta \mathcal{P}_i) + \alpha \partial_i \Delta \nabla \cdot \mathbf{P} \right) + \partial_i \Psi \quad (\text{S15})$$

or the Gaussian action,  $F_u^G$ , and to

$$\frac{\delta F_u}{\delta \mathcal{P}_i} = \frac{1}{\epsilon_0} \left( 2\gamma \mathcal{P}_i (\mathbf{P}^2 + P_0^2) - \kappa_l \partial_i \nabla \cdot \mathbf{P} + \kappa_t (\partial_i \nabla \cdot \mathbf{P} - \Delta \mathcal{P}_i) + \alpha \partial_i \Delta \nabla \cdot \mathbf{P} \right) + \partial_i \Psi \quad (\text{S16})$$

for the non Gaussian one,  $F_u$ :

In the two cases, we obtain

$$\psi = 0, \quad \mathbf{P} = 0. \quad (\text{S17})$$

The mean fields are vanishing both for Gaussian and non Gaussian configuration energy.

### S1.4. Gaussian susceptibility for an electrolyte

In this section we derive the expressions of the longitudinal  $\chi_{\parallel}^G(q)$  and transverse  $\chi_{\perp}^G(q)$  polarization susceptibility of an electrolyte.

We first define the total susceptibility of the system as

$$\chi_{\text{tot}}(\mathbf{r}_1 - \mathbf{r}_2) = \begin{pmatrix} \epsilon_0 \chi^G & \chi_{P,\psi}^G \\ \chi_{\psi,P}^G & \chi_{\psi,\psi}^G / \epsilon_0 \end{pmatrix} (\mathbf{r}_1 - \mathbf{r}_2) = \begin{pmatrix} \frac{\delta^2 F_u^G(\mathbf{P}, \Psi)}{\delta \mathcal{P}_i(\mathbf{r}_1) \delta \mathcal{P}_j(\mathbf{r}_2)} & \frac{\delta^2 F_u^G(\mathbf{P}, \Psi)}{\delta \mathcal{P}_i(\mathbf{r}_1) \delta \Psi(\mathbf{r}_1)} \\ \frac{\delta^2 F_u^G(\mathbf{P}, \Psi)}{\delta \Psi(\mathbf{r}_1) \delta \mathcal{P}_j(\mathbf{r}_2)} & \frac{\delta^2 F_u^G(\mathbf{P}, \Psi)}{\delta \Psi(\mathbf{r}_1) \delta \Psi(\mathbf{r}_2)} \end{pmatrix}^{-1} \quad (\text{S18})$$

with  $(\mathbf{P}, \psi)$  the mean fields minimizing the action  $F_u^G$ . Using the expressions given in Eq. (S4), we find for the inverse susceptibility of the system, in Fourier space,

$$\chi_{\text{tot}}^{-1}(\mathbf{q}) = \begin{pmatrix} & & & iq_x \\ & \chi_{\epsilon_0}^{-1G}(\mathbf{q}) & & iq_y \\ & & & iq_z \\ -iq_x & -iq_y & -iq_z & -(2ne^2\beta + \epsilon_0 q^2) \end{pmatrix}, \quad (\text{S19})$$

with the matrix  $\chi^{-1G}(\mathbf{q})$  given by

$$\chi_{ij}^{-1,G}(\mathbf{q}) = (K + \kappa_l q^2 + \alpha q^4) \frac{q_i q_j}{q^2} + (K + \kappa_t q^2) \left( \delta_{ij} - \frac{q_i q_j}{q^2} \right). \quad (\text{S20})$$

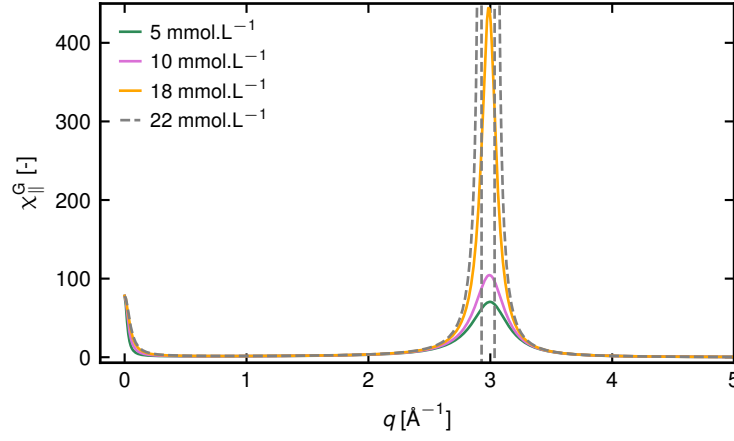

FIG. S2: Longitudinal susceptibility of electrolytes. The Gaussian susceptibility  $\chi_{||}^G(q)$  given in Eq. (S23), for increasing concentration. Parameters are given in caption of Fig. S1.

We inverse the matrix  $\chi_{\text{tot}}^{-1}(q)$  by using a block inversion and obtain

$$\chi_{\text{tot}}(\mathbf{q}) = \begin{pmatrix} \epsilon_0 \chi^G(\mathbf{q}) & iQ^\top \\ -iQ & \frac{\chi_{\psi,\psi}(q)}{\epsilon_0} \end{pmatrix} \quad (\text{S21})$$

with  $Q = (q_x, q_y, q_z)$  and

$$\chi_{ij}^G(\mathbf{q}) = \chi_{||}^G(q) \frac{q_i q_j}{q^2} + \chi_{\perp}^G(q) \left( \delta_{ij} - \frac{q_i q_j}{q^2} \right) \quad (\text{S22})$$

$$\chi_{||}^G(q) = \frac{\frac{\epsilon_w}{\lambda_D^2} + q^2}{\left( \frac{\epsilon_w}{\lambda_D^2} + q^2 \right) (K + \kappa_l q^2 + \alpha q^4) + q^2}, \quad \chi_{\perp}^G(q) = \frac{1}{K + \kappa_t q^2} \quad (\text{S23})$$

$$\chi_{\psi,\psi}(q) = -\frac{K + \kappa_l q^2 + \alpha q^4}{\left( \frac{\epsilon_w}{\lambda_D^2} + q^2 \right) (K + \kappa_l q^2 + \alpha q^4) + q^2} \quad (\text{S24})$$

where we have introduced the Debye length  $\lambda_D = \sqrt{\epsilon_0 \epsilon_w / 2\beta n e^2}$ . We plot the susceptibility  $\chi_{||}^G(q)$  for increasing concentrations ( $c = n/\mathcal{N}_a$ ,  $\mathcal{N}_a$  the Avogadro number) in Fig. S2. As we have ( $\kappa_l < 0$ ,  $\alpha > 0$ ) the denominator of  $\chi_{||}^G(q)$  will vanish for a small enough Debye length inducing a divergence of the susceptibility. See Fig. S2, grey dashed line. For the chosen set of parameters, the divergence occurs for  $c=22$  mmol.l<sup>-1</sup>. At this concentration, the longitudinal correlations are purely oscillating illustrating an unphysical crystalization of the medium.

### S1.5. Susceptibility for Gaussian model in real space

We express the Gaussian susceptibility  $\chi^G$  given in Eq. (S23) in real space. We perform the Fourier transform  $\chi_{ij}^G(\mathbf{r}) = \mathcal{F}_T(\chi_{ij}^G(\mathbf{q}))$  defined as

$$\chi_{ij}^G(\mathbf{r}) = \frac{1}{2\pi^3} \int_0^{2\pi} d\phi \int_0^\pi d\theta \sin(\theta) \int_0^\infty dq q^2 e^{iqr \cos(\theta)} \chi_{ij}^G(\mathbf{q}) \quad (\text{S25})$$

$\chi^G$  is here expressed in the intrinsic basis in which the vector  $\mathbf{r}$ , joining the two correlated points, is aligned with the  $\mathbf{e}_z$  direction of wavemode  $\mathbf{q}$  basis, as illustrated in Fig. S3. We develop the longitudinal projector  $q_i q_j / q^2$  ( $i, j = x, y, z$ ) in the spherical basis,

$$\frac{q_i q_j}{q^2} = \begin{pmatrix} \sin(\theta)^2 \cos(\phi)^2 & \sin(\theta)^2 \cos(\phi) \sin(\phi) & \sin(\theta) \cos(\theta) \cos(\phi) \\ \sin(\theta)^2 \cos(\phi) \sin(\phi) & \sin(\theta)^2 \sin(\phi)^2 & \sin(\theta) \cos(\theta) \sin(\phi) \\ \sin(\theta) \cos(\theta) \cos(\phi) & \sin(\theta) \cos(\theta) \sin(\phi) & \cos(\theta)^2 \end{pmatrix}, \quad (\text{S26})$$

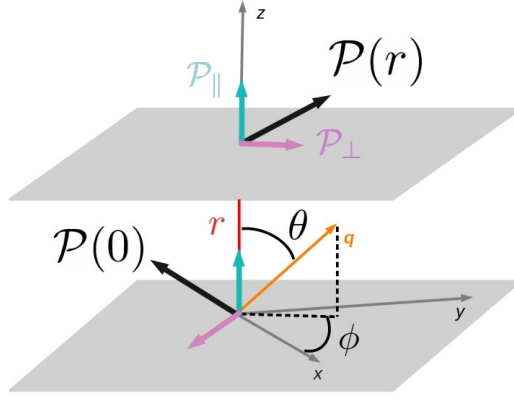

FIG. S3: Illustration of the basis considered to calculate the susceptibility tensor  $\chi^G$ .

Using Eqs. (S22,S23),  $\chi_{ij}^G(r)$  is splitted into two contributions:  $\chi_{ij}^G(r) = \mathcal{F}_T(\chi_{\parallel}^G(q)q_iq_j/q^2) + \mathcal{F}_T(\chi_{\perp}^G(q)(\delta_{ij} - q_iq_j/q^2))$ . We perform the integrals in Eq. (S25) using (S26). We get:

$$\mathcal{F}_T(\chi_{\parallel}^G(q)q_iq_j/q^2) = \begin{pmatrix} \frac{1}{2}(I_{1,\parallel}(r) - I_{2,\parallel}(r)) & 0 & 0 \\ 0 & \frac{1}{2}(I_{1,\parallel}(r) - I_{2,\parallel}(r)) & 0 \\ 0 & 0 & I_{2,\parallel}(r) \end{pmatrix}, \quad (\text{S27})$$

and

$$\mathcal{F}_T(\chi_{\perp}^G(q)(\delta_{ij} - q_iq_j/q^2)) = \begin{pmatrix} \frac{1}{2}(I_{1,\perp}(r) + I_{2,\perp}(r)) & 0 & 0 \\ 0 & \frac{1}{2}(I_{1,\perp}(r) + I_{2,\perp}(r)) & 0 \\ 0 & 0 & I_{1,\perp}(r) - I_{2,\perp}(r) \end{pmatrix}. \quad (\text{S28})$$

We have introduced four elementary functions ( $I_{\parallel,1}$ ,  $I_{\perp,1}$ ,  $I_{\parallel,2}$ ,  $I_{\perp,2}$ ), defined as follow:

$$\begin{aligned} I_{i,1}(r) &= \frac{1}{(2\pi)^3} \int_0^\infty dq q^2 \int_0^\pi d\theta \sin(\theta) \int_0^{2\pi} d\phi \chi_i^G(q) e^{iqr \cos(\theta)}, \\ I_{i,2}(r) &= \frac{1}{(2\pi)^3} \int_0^\infty dq \int_0^\pi d\theta \sin(\theta) \int_0^{2\pi} d\phi \chi_i^G(q) e^{iqr \cos(\theta)}, \end{aligned} \quad (\text{S29})$$

with  $i = \parallel, \perp$ . The Gaussian susceptibility finally reads

$$\chi^G(r) = \begin{pmatrix} \chi_{\perp}^G(r) & 0 & 0 \\ 0 & \chi_{\perp}^G(r) & 0 \\ 0 & 0 & \chi_{\parallel}^G(r) \end{pmatrix} \quad (\text{S30})$$

with

$$\chi_{\parallel}^G(r) = I_{2,\parallel}(r) + (I_{1,\perp}(r) - I_{2,\perp}(r)) \quad (\text{S31})$$

$$\chi_{\perp}^G(r) = \frac{I_{1,\parallel}(r) - I_{2,\parallel}(r)}{2} + \frac{I_{1,\perp}(r) - I_{2,\perp}(r)}{2} \quad (\text{S32})$$

in the basis  $\{\mathbf{e}_i\}$ ,  $i = x, y, z$  defined such that  $\mathbf{r}$  is aligned with  $\mathbf{e}_z$ . See sketch in Fig. S3.

The susceptibility associated with any distance vector  $\mathbf{r} = (x, y, z)$  is obtained by performing the following change of basis:

$$\chi_{\text{cart}}^G = R^{-1} \cdot \chi^G(r) \cdot R, \quad (\text{S33})$$

$R$  being the change-of-basis matrix from Cartesian to spherical coordinates.

### S1.6. One-loop free energy expansion

The partition function can be expanded to the second order around the mean field point  $(\mathbf{P}, \psi)$ , as

$$\begin{aligned}\Xi &\approx e^{-\beta F_u[\mathbf{P}, \psi]} \int \mathcal{D}[\delta \mathbf{P}] \mathcal{D}[\delta \Psi] e^{-\frac{\beta}{2} \int d\mathbf{r} d\mathbf{r}' (\delta \mathbf{P}(\mathbf{r}), \delta \Psi(\mathbf{r})) \cdot F_u^{(2)}(\mathbf{P}, \psi) \cdot (\delta \mathbf{P}(\mathbf{r}'), \delta \Psi(\mathbf{r}'))} \\ &= e^{-\beta F_u[\psi, P]} \left( \beta |F_u^{(2)}| \right)^{-1/2}\end{aligned}\quad (\text{S34})$$

where we have dropped the prefactor.  $F_u^{(2)}(\mathbf{r} - \mathbf{r}')$  is the second functional derivative of the action and can be defined as follows:

$$F_u^{(2)}(\mathbf{r} - \mathbf{r}') = \begin{pmatrix} \frac{\delta^2 F_u(\mathbf{P}, \psi)}{\delta \mathcal{P}_i(\mathbf{r}) \delta \mathcal{P}_j(\mathbf{r}')} & \frac{\delta^2 F_u(\mathbf{P}, \psi)}{\delta \mathcal{P}_i(\mathbf{r}) \delta \Psi(\mathbf{r}')} \\ \frac{\delta^2 F_u(\mathbf{P}, \psi)}{\delta \Psi(\mathbf{r}) \delta \mathcal{P}_i(\mathbf{r}')} & \frac{\delta^2 F_u(\mathbf{P}, \psi)}{\delta \Psi(\mathbf{r}) \delta \Psi(\mathbf{r}')} \end{pmatrix} \quad (\text{S35})$$

with

$$\frac{\delta F_u(\mathbf{P}, \psi)}{\delta \Psi(\mathbf{r}) \delta \Psi(\mathbf{r}')} = (\epsilon_0 \Delta_{\mathbf{r}} - 2\Lambda \beta e^2 \cosh(\beta e \psi)) \delta(\mathbf{r} - \mathbf{r}') \quad (\text{S36})$$

$$\frac{\delta F_u(\mathbf{P}, \psi)}{\delta \mathcal{P}_i(\mathbf{r}) \delta \mathcal{P}_j(\mathbf{r}')} = \frac{1}{\epsilon_0} \left( 2\gamma (P_{ij}^2 + P_0^2) \delta_{ij} + 4\gamma P_i P_j - \kappa_l \partial_i \partial_j + \kappa_t (\partial_i \partial_j - \Delta \delta_{ij}) + \alpha \Delta \partial_i \partial_j \right) \delta(\mathbf{r} - \mathbf{r}') \quad (\text{S37})$$

$$\frac{\delta F_u(\mathbf{P}, \psi)}{\delta \Psi(\mathbf{r}) \delta \mathcal{P}_i(\mathbf{r}')} = -\partial_i \delta(\mathbf{r} - \mathbf{r}'), \quad \frac{\delta F_u(\mathbf{P}, \psi)}{\delta \mathcal{P}_i(\mathbf{r}) \delta \Psi(\mathbf{r}')} = \partial_i \delta(\mathbf{r} - \mathbf{r}') \quad (\text{S38})$$

We set  $2\gamma P_0^2 = K$  so that the Gaussian asymptotic behavior of the  $P^4$ -model, reached in the low polarization limit, is similar to the Gaussian model. The Gibbs free energy at the first order with a loop expansion can be written as:

$$\mathcal{F} \approx F_u[\mathbf{P}, \psi] + \frac{1}{2\beta} \text{Tr} \ln \beta F_u^{(2)}[\mathbf{P}, \psi]. \quad (\text{S39})$$

### S1.7. One-loop correction for the inverse susceptibility

In this subsection, we expand the inverse polarization susceptibility to the first order,  $\chi^{-1} \approx \chi^{-1, G} + \chi^{-1, 1}$ . Using its expression as a function of the Gibbs free energy of the system,

$$\frac{1}{\epsilon_0} \chi_{ij}^{-1}(\mathbf{r}_1 - \mathbf{r}_2) = \frac{\delta^2 \mathcal{F}(\mathbf{P}, \psi)}{\delta \mathcal{P}_i(\mathbf{r}_1) \delta \mathcal{P}_j(\mathbf{r}_2)} \quad (\text{S40})$$

and the first order expansion of  $\mathcal{F}$ , (Eq. S39), we get:

$$\begin{aligned}\frac{1}{\epsilon_0} \chi_{xx}^{-1, 1}(\mathbf{r}_1 - \mathbf{r}_2) &= \frac{\delta \text{Tr} \ln(\beta F_u^{(2)})}{\delta \mathcal{P}_x(\mathbf{r}_1) \delta \mathcal{P}_x(\mathbf{r}_2)}(\mathbf{P}, \psi) \\ &= \text{Tr} \left( \left( F_u^{(2)} \right)^{-1} \cdot \frac{\partial^2 F_u^{(2)}}{\partial \mathcal{P}_x(\mathbf{r}_1) \partial \mathcal{P}_x(\mathbf{r}_2)} - \frac{\delta F_u^{(2)}}{\delta \mathcal{P}_x(\mathbf{r}_1)} \frac{\delta F_u^{(2)}}{\delta \mathcal{P}_x(\mathbf{r}_2)} \cdot \left( F_u^{(2)} \right)^{-2} \right) (\mathbf{P}, \psi).\end{aligned}\quad (\text{S41})$$

The second matrix product in the right hand term is vanishing as  $\delta F_u^{(2)} / \delta \mathcal{P}_x(\mathbf{r}_2)(\mathbf{P}, \psi) = 0$ . We thus get:

$$\frac{\delta \text{Tr} \ln(\beta F_u^{(2)})}{\delta \mathcal{P}_x(\mathbf{r}_1) \delta \mathcal{P}_x(\mathbf{r}_2)}(\mathbf{P}, \psi) = \text{Tr} \left( \left( F_u^{(2)} \right)^{-1} \cdot \frac{\partial^2 F_u^{(2)}}{\partial \mathcal{P}_x(\mathbf{r}_1) \partial \mathcal{P}_x(\mathbf{r}_2)} \right) (\mathbf{P}, \psi). \quad (\text{S42})$$

We use the expression of  $F_u^{(2)}$  given in Eq. (S37) and obtain

$$\frac{\partial^2 F_u^{(2)}(\mathbf{P}, \psi)}{\partial \mathcal{P}_x(\mathbf{r}_1) \partial \mathcal{P}_x(\mathbf{r}_2)} = \begin{pmatrix} 12\gamma/\epsilon_0 & 0 & 0 & 0 \\ 0 & 4\gamma/\epsilon_0 & 0 & 0 \\ 0 & 0 & 4\gamma/\epsilon_0 & 0 \\ 0 & 0 & 0 & 0 \end{pmatrix} \delta(\mathbf{r} - \mathbf{r}_1) \delta(\mathbf{r} - \mathbf{r}_2) \delta(\mathbf{r}' - \mathbf{r}) \quad (\text{S43})$$

and

$$\frac{\partial^2 F_u^{(2)}(\mathbf{P}, \psi)}{\partial P_x(\mathbf{r}_1) \partial P_y(\mathbf{r}_2)} = \begin{pmatrix} 0 & 4\gamma/\epsilon_0 & 0 & 0 \\ 4\gamma/\epsilon_0 & 0 & 0 & 0 \\ 0 & 0 & 0 & 0 \\ 0 & 0 & 0 & 0 \end{pmatrix} \delta(\mathbf{r} - \mathbf{r}_1) \delta(\mathbf{r} - \mathbf{r}_2) \delta(\mathbf{r}' - \mathbf{r}) \quad (\text{S44})$$

The other matrices are easily deduced by symmetry.

We now have to calculate the trace of matrices in (S43) by integrating over the continuous indices  $\int d\mathbf{r} d\mathbf{r}'$  and summing over the discrete indices. The polarization correlations depend only on the distance  $u = |\mathbf{r} - \mathbf{r}'|$ . We thus write:

$$\int d\mathbf{r} d\mathbf{r}' \left(F_u^{(2)}\right)^{-1} \cdot \frac{\partial^2 F_u^{(2)}}{\partial \mathcal{P}_i(\mathbf{r}_1) \partial \mathcal{P}_j(\mathbf{r}_2)} = \int d\mathbf{r} \int du u^2 \left( \int d\phi d\theta \sin(\theta) \left(F_u^{(2)}\right)^{-1} \right) \frac{\partial^2 F_u^{(2)}}{\partial \mathcal{P}_i(\mathbf{r}_1) \partial \mathcal{P}_j(\mathbf{r}_2)} \quad (\text{S45})$$

Using  $\delta(\mathbf{r} - \mathbf{r}') = \delta(u)/2\pi u^2$  and  $\left(F_u^{(2)}\right)^{-1}(\mathbf{P}, \psi) = \chi_{\mathbf{P}, \psi}^G(\mathbf{r} - \mathbf{r}')$  given in Eq. (S40), we perform the integral over  $\theta$  and  $\phi$  and find for the polarization correlation:

$$\int_0^{2\pi} d\phi \int_0^\pi d\theta \sin(\theta) R^{-1} \cdot \chi_{ij}^G(u) \cdot R = \frac{4\pi}{3} (\chi_{\parallel}(u) + 2\chi_{\perp}(u)) \delta_{ij}. \quad (\text{S46})$$

We now perform the matrix product of matrix given in Eqs. (S43, S46), calculate its trace and find:

$$\begin{aligned} \chi_{x,x'}^{-1,1}(\mathbf{r}_1 - \mathbf{r}_2) &= \frac{\pi}{\beta} \int d\mathbf{r} \int_0^\infty du 4\gamma\epsilon_0 \left( \frac{10}{3} \chi_{\parallel}^G(u) + \frac{20}{3} \chi_{\perp}^G(u) \right) \frac{\delta(u)}{2\pi} \delta(\mathbf{r} - \mathbf{r}_1) \delta(\mathbf{r} - \mathbf{r}_2) \\ &= \frac{20\gamma\epsilon_0}{3\beta} (\chi_{\parallel}^G(0) + 2\chi_{\perp}^G(0)) \delta(\mathbf{r}_1 - \mathbf{r}_2). \end{aligned} \quad (\text{S47})$$

Note that we find the same value for  $\chi_{yy}^{-1,1}$  and  $\chi_{zz}^{-1,1}$  and that the cross terms are vanishing. We calculate the susceptibility at  $r = 0$ ,  $\chi^G(0)$ , using the elementary functions defined in Eq. (S29) and taken in 0 as follows,

$$I_{1,\parallel}(0) = \frac{1}{2\pi^2} \int_0^\infty dq q^2 \frac{\epsilon_w/\lambda_D^2 + q^2}{(\epsilon_w/\lambda_D^2 + q^2)(K + \kappa_l q^2 + \alpha q^4) + q^2}, \quad (\text{S48})$$

$$I_{1,\perp}(r_c) = \frac{1}{2\pi^2} \int_0^{2\pi/r_c} dq \frac{q^2}{K + \kappa_l q^2} = \frac{1}{\pi K \lambda_t^2 r_c} \quad (\text{S49})$$

$$I_{2,\parallel}(0) = \frac{I_{1,\parallel}(0)}{3}, \quad I_{2,\perp}(0) = \frac{I_{1,\perp}(r_c)}{3} \quad (\text{S50})$$

where we have introduced a cutoff length  $r_c$  to remove the divergence for  $I_{1/2,\perp}$  in  $r = 0$ .

The Gaussian susceptibility tensor reads,

$$\chi_{\parallel}^G(r_c) = I_{2,\parallel}(0) + I_{1,\perp}(r_c) - I_{2,\perp}(r_c), \quad \chi_{\perp}^G(r_c) = \frac{1}{2} (I_{1,\parallel}(0) - I_{2,\parallel}(0) + I_{1,\perp}(r_c) - I_{2,\perp}(r_c)). \quad (\text{S51})$$

Using Eq. (S47), we obtain in Fourier space,

$$\chi^{-1,1}(\mathbf{q}) = \delta K \frac{q_i q_j}{q^2} + \delta K \left( \delta_{ij} - \frac{q_i q_j}{q^2} \right), \quad \text{with} \quad \delta K = \frac{20\gamma\epsilon_0}{3\beta} (\chi_{\parallel}^G(r_c) + 2\chi_{\perp}^G(r_c)). \quad (\text{S52})$$

Finally, we get the expression for the inverse polarization susceptibility at the first order,

$$\chi_{ij}^{-1}(\mathbf{q}) = (K + \delta K + \kappa_l q^2 + \alpha q^4) \frac{q_i q_j}{q^2} + (K + \delta K + \kappa_l q^2) \left( \delta_{ij} - \frac{q_i q_j}{q^2} \right). \quad (\text{S53})$$

where we have used the expression of  $\chi^G(\mathbf{q})$  given in Eq. (S20).

### S1.8. Linear dependence of $\chi^{-1,1}(q)$ in salt concentration $c$

The correction  $\delta K$  is now splitted into two contributions,

$$\delta K = \delta K_w + \delta K_{c,c} + \tau(c^2) \quad (\text{S54})$$

a pure water one  $\delta K_w$  and a second one,  $\delta K_{c,c}$  depending on the salt concentration and expanded linearly in  $c$ .

To get explicit expression of  $\delta K_w$  and  $\delta K_{c,c}$ , we expand linearly in  $c$  the functions  $I_{i,x}(0)$ ,  $i = 1, 2$ ,  $x = \parallel, \perp$  given in Eq. (S48-S50), using  $\epsilon_w/\lambda_D^2 = c \times 2\mathcal{N}_a e^2 \beta / \epsilon_0$ . We get

$$I_{i,\parallel}(0) = I_{i,\parallel}^w(0) + c \times I_{i,\parallel}^1(0) + \tau(c^2) \quad (\text{S55})$$

$$I_{i,\perp}(r_c) = I_{i,\parallel}^w(r_c), \quad i = 1, 2 \quad (\text{S56})$$

in which the functions are split into a pure water contribution and a linear correction in  $c$ . Note that  $I_{i,\perp}$  functions do not depend of the salt concentration, the associated salt correction is thus vanishing.

The functions for pure water obey

$$I_{1,\parallel}^w(0) = \frac{1}{2\pi^2} \int_0^\infty dq q^2 \frac{1}{1 + K + \kappa_l q^2 + \alpha q^4}, \quad I_{2,\parallel}^w(0) = \frac{I_{1,\parallel}^w(r_c)}{3}, \quad (\text{S57})$$

$$I_{1,\perp}^w(0) = \frac{1}{2\pi^2} \int_0^{\frac{2\pi}{r_c}} dq q^2 \frac{1}{K + \kappa_t q^2}, \quad I_{2,\perp}^w(r_c) = \frac{I_{1,\perp}^w(r_c)}{3}, \quad (\text{S58})$$

and the linear correction for the parallel function,

$$I_{1,\parallel}^1(0) = \frac{1}{2\pi^2 \epsilon_0} \int_0^\infty dq \frac{2\mathcal{N}_a e^2 \beta}{(1 + K + \kappa_l q^2 + \alpha q^4)^2}, \quad I_{2,\parallel}^1(0) = \frac{I_{1,\parallel}^1(0)}{3}. \quad (\text{S59})$$

The expression of  $\chi_{\parallel}^w(r_c)$  and  $\chi_{\perp}^w(r_c)$  are obtained by replacing  $I_{i,\parallel}(0)$  by  $I_{i,\parallel}^w(0)$  and  $I_{i,\perp}(0)$  by  $I_{i,\perp}^w(0)$  in Eq. (S47). Finally, we get:

$$\delta K_w = \frac{20\gamma\epsilon_0}{3\beta} \left( \chi_{\parallel}^w(r_c) + \chi_{\perp}^w(r_c) \right). \quad (\text{S60})$$

We set  $\delta K_w$  to zero as it is included in the fitted parameter  $K$ . Using the expressions of  $\delta K$  in Eq. (S52) and  $(\chi_{\perp}^G, \chi_{\parallel}^G)$  in Eq. (S51), we obtain

$$\delta K_c = \frac{20\gamma\epsilon_0}{3\beta} I_{1,\parallel}(0). \quad (\text{S61})$$

We perform the integral in Eq. (S59) and obtain

$$I_{1,\parallel}^1(0) = \frac{\beta \mathcal{N}_a e^2 (\epsilon_w - 1)^2}{64\pi \epsilon_0 \epsilon_w} \frac{(4\pi^2 \lambda_d^2 + \lambda_o^2)(4\pi^2 \lambda_d^2 + 5\lambda_o^2)}{\lambda_d \lambda_o^4} \quad (\text{S62})$$

after having expressed  $K$ ,  $\kappa_l$ ,  $\alpha$  as functions of  $\epsilon_w$ ,  $\lambda_o$ ,  $\lambda_d$  by inverting Eq. (S5). We deduce that,

$$\delta K_c = \gamma \frac{5\mathcal{N}_a e^2 (\epsilon_w - 1)^2}{24\pi \epsilon_w} \frac{(4\pi^2 \lambda_d^2 + \lambda_o^2)(4\pi^2 \lambda_d^2 + 5\lambda_o^2)}{\lambda_d \lambda_o^4} \quad (\text{S63})$$

Expanding linearly the relation  $\epsilon(c) = 1 + 1/(K + \delta K_{c,c})$ , we obtain for the permittivity of the electrolytes

$$\epsilon(c) = \epsilon_w - \frac{\delta K_c}{K^2} c. \quad (\text{S64})$$

The inverse susceptibility can thus be written as:

$$\begin{aligned} \chi^{-1}(q) &= \chi^{-1,G}(q) + \chi^{-1,1}(q) \\ &= (K + \delta K_{c,c} + \kappa_l q^2 + \alpha q^4) \frac{q_i q_j}{q^2} + (K + \delta K_{c,c} + \kappa_t q^2) \left( \delta_{ij} - \frac{q_i q_j}{q^2} \right). \end{aligned} \quad (\text{S65})$$

that is inverted to get the one-loop corrected susceptibility

$$\chi_{\parallel}(q) = \frac{1}{1 + K + \delta K_{c,c} + \kappa_l q^2 + \alpha q^4} \quad (\text{S66})$$

which we plot for increasing salt concentration in Fig. S4. One sees comparing the susceptibilities obtained for the Gaussian model plotted in Fig. S2 and the one-loop expanded one plotted in Fig (S5) that the enhancement of the pseudo-resonant peak at  $q=3 \text{ \AA}^{-1}$  is attenuated but not canceled by the one-loop correction.

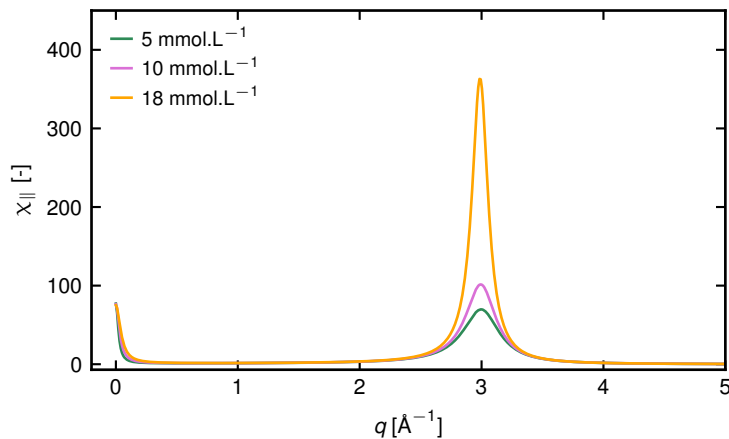

FIG. S4: One-loop expanded longitudinal susceptibility of electrolytes. The susceptibility  $\chi_{||}(q)$  given in Eq. (S66), for increasing concentration with  $\delta K_c = 0.028 \text{ mol}^{-1} \cdot \text{L}$ . Other parameters are given in caption of Fig. S1.

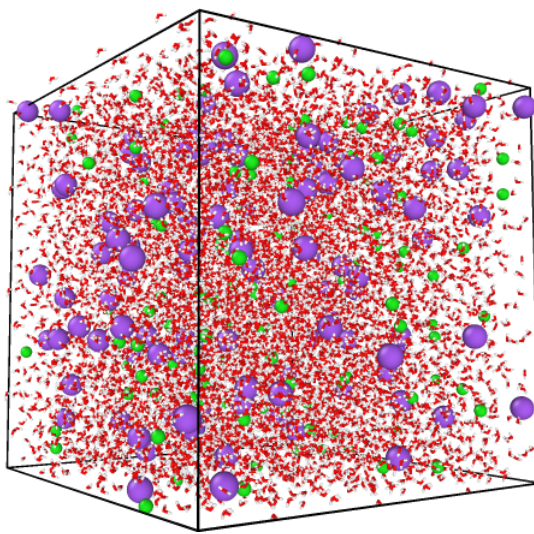

FIG. S5: Snapshot of a simulation box of electrolytes. Red and white sticks represent TIP4p/ε water molecules, purple spheres chloride  $\text{Cl}^-$  ions and green spheres sodium  $\text{Na}^+$  ions. This picture corresponds to a  $0.75 \text{ mol.l}^{-1}$  solution. Side size of the box:  $L=6.5 \text{ nm}$ .

## S2. SUPPLEMENTARY INFORMATION FOR MOLECULAR DYNAMIC SIMULATION

### S2.1. Methods

*a. Molecular dynamics simulations* We simulate a cubic water box of side size  $L=6.5 \text{ nm}$  composed of  $N_w$  water molecules,  $N_w$  going from 9033 to 8527 for increasing salt concentration. See a snapshot of the simulated system in Fig. S5. The  $0.15 \text{ mol.l}^{-1}$  solution contains 25 ion pairs, the  $0.75 \text{ mol.l}^{-1}$  solution contains 124 ion pairs and the  $1.5 \text{ mol.l}^{-1}$  solution, 248 ion pairs. Simulations are performed using GROMACS 2021 molecular dynamics simulation package ([7]), the integration time steps is set to  $\Delta t=2 \text{ fs}$ . Simulation boxes are periodically replicated in all directions and long range electrostatics are handled using the smooth particle mesh Ewald (SPME) technique. Lennard-Jones interactions are cut off at a distance  $r_{\text{cut}}=0.9 \text{ nm}$ . A potential shift is used at the cut-off distance. All systems are coupled to a heat bath at 300 K using v-rescale thermostat with a time constant of 0.5 ps. We use MDAnalysis to treat the trajectories. After creating the simulation box, we perform a first energy minimization. We equilibrate the system in the NVT ensemble for 200 ps, and afterwards in the NPT ensemble for another 200 ps using a Berendsen barostat at 1 bar. Production runs are performed in the NVT ensemble for 20 ns.

We perform simulations with TIP4p/ε ([2]), a 4 interaction site, three point-charges and one Lennard Jones

reference site model. The Lenard-Jones (LJ) center is placed on the oxygen. Charges are placed on the hydrogen atoms and on an additional interaction site, M, carrying the negative charge. The ions ( $\text{Na}^+$  and  $\text{Cl}^-$ ) were treated according to the force field developed in the reference [8].

*b. Statistical treatment* For the longitudinal and transverse susceptibility, the error bars are derived following the reblocking method [9]. For the bulk permittivity, we cut the trajectory in 5 statistically independent blocks, compute the bulk permittivity of each block, estimate the sample variance  $\sigma^2$  and define the error bar as  $\sqrt{\sigma^2/5}$ .

*c. Permittivity* Bulk permittivity is calculated from the total system dipole moments [10]  $\mathbf{M}$  according to:

$$\chi = \frac{\langle \mathbf{M} \cdot \mathbf{M} \rangle - \langle \mathbf{M} \rangle \cdot \langle \mathbf{M} \rangle}{3\epsilon_0 k_B T V}, \quad (\text{S67})$$

as implemented in the GROMACS dipoles module.  $\mathbf{M}$  is the volume integral of the polarization as  $\mathbf{M} = \int_V d\mathbf{r} \mathbf{P}(\mathbf{r})$  and  $V$  is the volume of the box. Note that the ion polarization is not taken into account.

*d. Susceptibilities* To compute the  $q$ -dependent susceptibilities, we use the fluctuation-dissipation theorem, relating the response functions to the polarization fluctuations as follows:

$$\chi_{ij}(\mathbf{q}) = \frac{\langle \mathbf{P}(\mathbf{q}) \cdot \mathbf{P}(-\mathbf{q}) \rangle}{\epsilon_0 k_B T} \quad (\text{S68})$$

One can express the longitudinal susceptibility as a function of the charge structure factor  $S(q)$  and gets

$$\chi_{\parallel}(q) = \frac{S(q)}{q^2 \epsilon_0 k_B T} \quad (\text{S69})$$

The charge structure factor in the Fourier space can be decomposed into a intramolecular and intermolecular part,

$$S(q) = S_{\text{int}}(q) + S_{\text{inter}}(q) \quad (\text{S70})$$

with  $S_{\text{inter}}(q)$  the intermolecular contribution

$$S_{\text{inter}}(q) = \frac{4n_w z^2 e^2}{q^2} (h_{\text{MM}}(q) + h_{\text{HH}}(q) - 2h_{\text{HM}}(q)) \quad (\text{S71})$$

$z$  is the valency,  $e$  being the elementary charge,  $n_w$  the molecular number density.  $h_{\text{IJ}}$  is the Fourier transform of  $g_{\text{IJ}}(r) - 1$ ,  $g_{\text{IJ}}(r)$  being the radial distribution function associated with the atoms couple IJ. The intramolecular contribution can be written as

$$S_{\text{intra}}(q) = \frac{4n_w z^2 e^2}{q^2} \left( \frac{\sin(qd_{\text{HH}})}{qd_{\text{HH}}} - 4 \frac{\sin(qd_{\text{HM}})}{qd_{\text{HM}}} + 3 \right) \quad (\text{S72})$$

where  $d_{\text{IJ}}$  is the intramolecular distance between atom I and J.

At low  $q$  the precision of this expression of the structure factor become pretty low as the function  $h_{\text{IJ}}(r)$  is obtained on a finite range imposed by the box size. To solve this problem, we proceed as follows. For  $q < 2.5 \text{ \AA}^{-1}$ , we take into account the periodicity of the system, calculate the charge structure factor for discretized values of the wave length  $q$ ,  $q = 2\pi/L\sqrt{n_x^2 + n_y^2 + n_z^2}$ . We compute directly the charge structure factor from the charge distribution  $\tilde{\rho}(q)$  in the Fourier space,

$$\tilde{\rho}(q) = \sum_{i=1}^{N_w} e z e^{i\mathbf{q} \cdot \mathbf{r}} (-2e^{-i\mathbf{q} \cdot \mathbf{r}_{\text{M},i}} + e^{-i\mathbf{q} \cdot \mathbf{r}_{\text{H1},i}} + e^{-i\mathbf{q} \cdot \mathbf{r}_{\text{H2},i}}) \quad (\text{S73})$$

where  $\text{H}_{1,i}$  and  $\text{H}_{2,i}$  stand for the two hydrogens of the molecule  $j$ . the charge structure factor  $S(q) = \langle \tilde{\rho}(q) \tilde{\rho}(-q) \rangle / V$ ,

$$\begin{aligned} S(q) = \frac{2q_H^2}{V} \sum_{i,j,j \leq i} & \left( 4 \cos(\mathbf{q} \cdot \mathbf{d}_{\text{OiOj}}) - 2 \cos(\mathbf{q} \cdot \mathbf{d}_{\text{OiH1j}}) - 2 \cos(\mathbf{q} \cdot \mathbf{d}_{\text{H1iOj}}) \right. \\ & - 2 \cos(\mathbf{q} \cdot \mathbf{d}_{\text{OiH2j}}) - 2 \cos(\mathbf{q} \cdot \mathbf{d}_{\text{H2iOj}}) + \cos(\mathbf{q} \cdot \mathbf{d}_{\text{H1iH1j}}) + \cos(\mathbf{q} \cdot \mathbf{d}_{\text{H2iH2j}}) \\ & \left. + \cos(\mathbf{q} \cdot \mathbf{d}_{\text{H1iH2j}}) + \cos(\mathbf{q} \cdot \mathbf{d}_{\text{H2iH1j}}) \right) \end{aligned} \quad (\text{S74})$$

where  $q$  is a vector and  $d_{A_i A_j}$  stands for  $\mathbf{r}_{A_i} - \mathbf{r}_{A_j}$ .

The transverse susceptibility is performed following ([11]). The polarization of the medium in the Fourier space

$$\mathbf{P}(\mathbf{q}) = \sum_j \mathbf{p}_j(\mathbf{q}) e^{-i\mathbf{q} \cdot \mathbf{r}_j} \quad (\text{S75})$$

can be written as a sum over the molecular polarization  $\mathbf{p}_j(\mathbf{q})$  of the molecule  $j$  which reads as

$$\mathbf{p}_j(\mathbf{q}) = \frac{1}{\sqrt{V}} \sum_{\alpha} \frac{e z_{\alpha} \delta \mathbf{r}_{\alpha j}}{i \mathbf{q} \cdot \delta \mathbf{r}_{\alpha j}} (1 - e^{-i\mathbf{q} \cdot \delta \mathbf{r}_{\alpha j}}) \quad (\text{S76})$$

with  $\delta \mathbf{r}_{\alpha j}$  the distance between the charge  $\alpha$  and the center of mass of the molecule and  $V$  the volume of the simulation box. We then take the transverse part of the polarization  $\mathbf{P}_{\perp}(\mathbf{q}) = \mathbf{q} \times \mathbf{P}(\mathbf{q})/q$  and define the transverse susceptibility as

$$\chi_{\perp}(q) = \frac{\langle \mathbf{P}_{\perp}(\mathbf{q}) \cdot \mathbf{P}_{\perp}(-\mathbf{q}) \rangle}{2k_B T \epsilon_0}. \quad (\text{S77})$$

Note that we replace  $(1 - e^{-i\mathbf{q} \cdot \delta \mathbf{r}_{\alpha j}})/i\mathbf{q} \cdot \delta \mathbf{r}_{\alpha j}$  by 1 for  $\mathbf{q} \cdot \delta \mathbf{r}_{\alpha j} < 10^{-5}$  to prevent numerical errors.

- 
- [1] A. C. Maggs and R. Everaers. Simulating nanoscale dielectric response. *Phys. Rev. Lett.*, 96:230603, 2006.
  - [2] R. Fuentes-Azcatl and J. Alejandre. Non-Polarizable Force Field of Water Based on the Dielectric Constant: TIP4P. *J. Phys. Chem. B*, 118:1263–1272, 2014.
  - [3] P. A. Bopp, A. A. Kornyshev, and G. Sutmann. Static Nonlocal Dielectric Function of Liquid Water. *Phys. Rev. Lett.*, 76:1280–1283, 1996.
  - [4] A. A. Kornyshev, S. Leikin, and G. Sutmann. "Overscreening" in a polar liquid as a result of coupling between polarization and density fluctuations. *Electrochimica Acta*, 42:849–865, 1997.
  - [5] H. Berthoumieux and A. C. Maggs. Fluctuation-induced forces governed by the dielectric properties of water- a contribution to the hydrophobic interaction. *J. Chem. Phys.*, 143:104501, 2015.
  - [6] A. Levy, D. Andelman, and H. Orland. Dielectric constant of ionic solutions: A field-theory approach. *Phys. Rev. Lett.*, 108:227801, 2012.
  - [7] M. J. Abraham, T. Murtola, R. Schulz, S. Páll, J. C. Smith, B. Hess, and E. Lindahl. GROMACS: High performance molecular simulations through multi-level parallelism from laptops to supercomputers. *SoftwareX*, 1-2:19–25, 2015.
  - [8] P. Loche, P. Steinbrunner, S. Friedowitz, R. R. Netz, and D. J. Bonhuis. Transferable Ion Force Fields in Water from a Simultaneous Optimization of Ion Solvation and Ion-Ion Interaction. *J. Phys. Chem. B*, 125:8581–8587, 2021.
  - [9] H. Flyvbjerg and H. G. Peetersen. Error estimates on averages of correlated data. *J. Chem. Phys.*, 91:461, 1989.
  - [10] M. Neumann. Dipole moment fluctuation formulas in computer simulations of polar systems. *Mol. Phys.*, 50:841–858, 1983.
  - [11] P. A. Bopp, A. A. Kornyshev, and G. Sutmann. Frequency and wave-vector dependent dielectric function of water: Collective modes and relaxation spectra. *J. Chem. Phys.*, 109:1940–1958, 1998.
